# Supplementary material for: A Tracer-Based Algorithm for Automatic Generation of Seafloor Age Grids from Plate Tectonic Reconstructions
Source: arXiv:1910.03351 source file (2019-10-08)
Supplement: Supplementary file 1 [file supplemental_materials.pdf]

# Supplemental Material

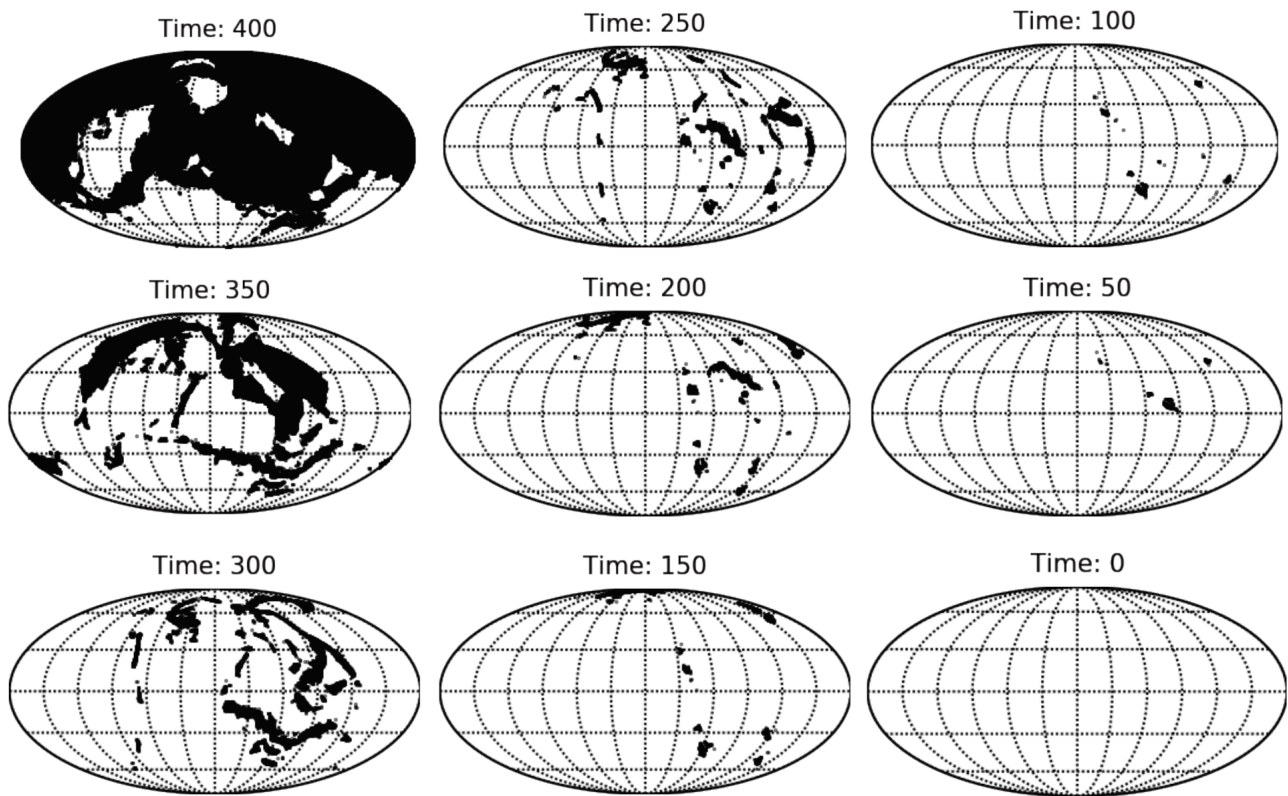

**Figure S1:** Maps showing the effect of an initial condition applied at 400 Ma. Dark regions represent the area covered by the initially added tracers through time.

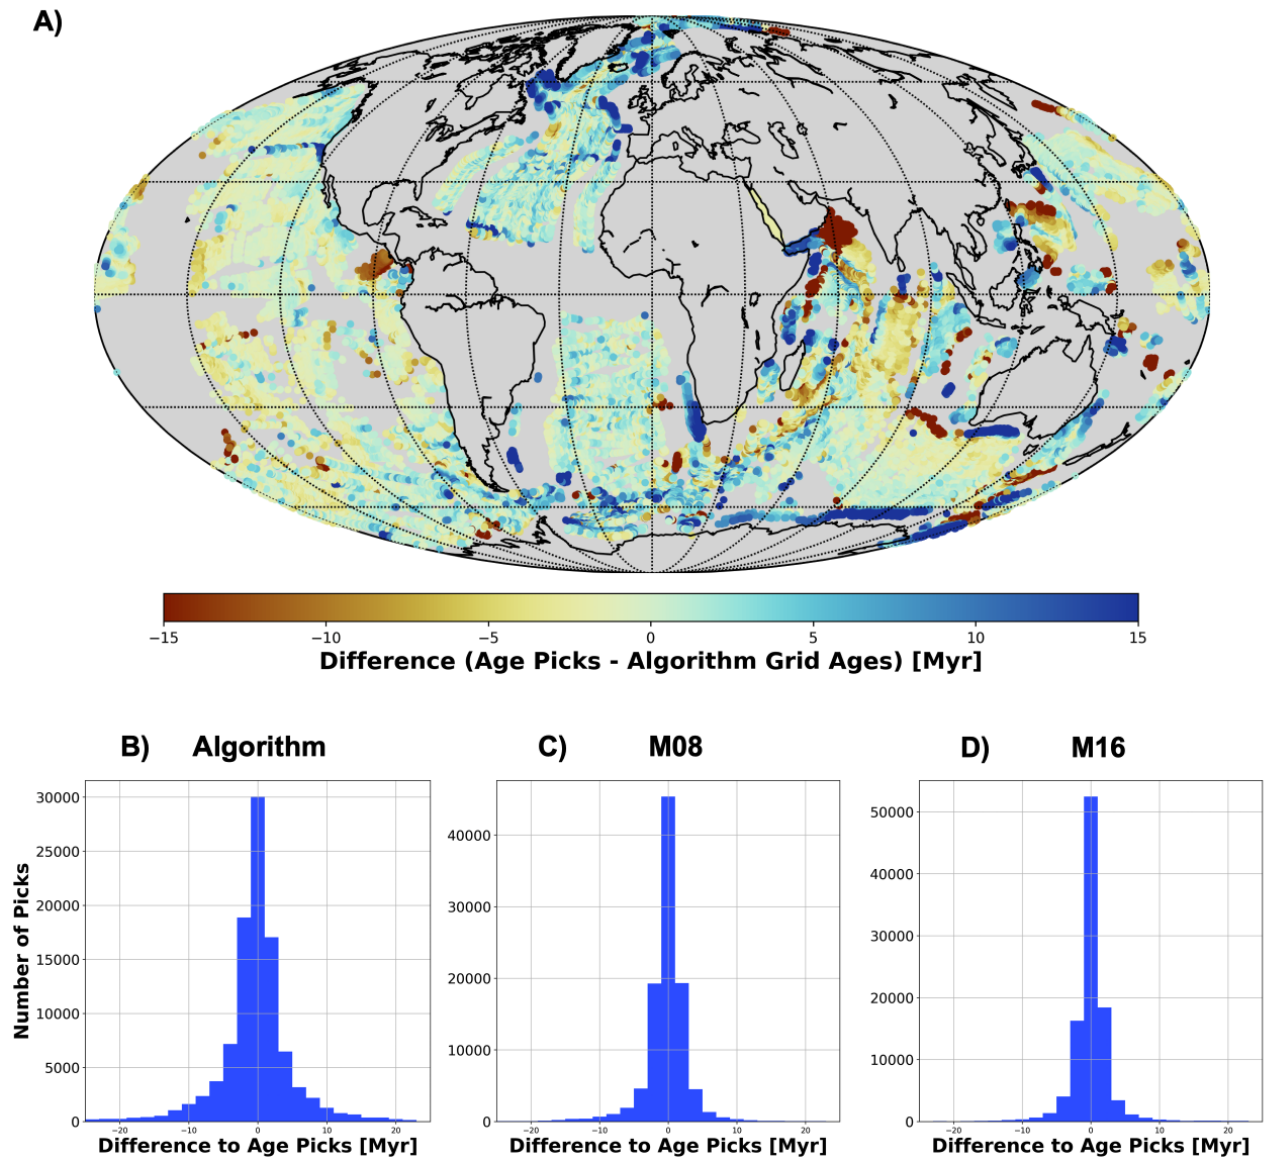

**Figure S2:** Map (A) comparing our automatic algorithm generated present-day age grid to ages inferred from magnetic reversal picks. Distributions (B-D) show the number of pick ages that fall within a certain deviation from the grid ages they are compared to. The total number of pick ages are 101418. The three age grid models used for comparison are: (B) our algorithm generated age grid, (C) M08 - Muller et al., 2008b and (D) M16 - Muller et al., 2016.
